# Supplementary material for: Steer, Don't Solve: Training Small Critic Models for Large Code Agents
Source: arXiv:2606.21811 source file (2026-09-01)
Supplement: Supplementary file 1 [file appendix_fallback_full.tex]

\section{Opus Teacher Critic Ablation}
\label{app:fallback_full}

\providecommand{\dup}[1]{\textcolor{darkgreen}{\scriptsize($\uparrow$#1)}}
\providecommand{\ddn}[1]{\textcolor{red}{\scriptsize($\downarrow$#1)}}
\providecommand{\dupR}[1]{\textcolor{red}{\scriptsize($\uparrow$#1)}}
\providecommand{\ddnG}[1]{\textcolor{darkgreen}{\scriptsize($\downarrow$#1)}}
\providecommand{\dzero}{\textcolor{darkgreen}{\scriptsize(0.0)}}

Table~\ref{tab:fallback_full} sweeps the \opus{} teacher critic across both prompt formats (high-level / detailed), both intervention intervals ($k\in\{5,10\}$), and both fallback states on the \cwm{} agent. The other critic conditions (no-critic baselines, the untrained \qwenEightB{} critic, and our trained critic) are reported across all three agent models in App.~\ref{app:fallback_triagent}; here we hold the agent fixed and isolate the teacher's prompt and budget axes. Arrows are vs.\ the matching no-critic row at the same fallback state.

\begin{table*}[t]
\centering
\footnotesize
\setlength{\tabcolsep}{2pt}
\resizebox{\textwidth}{!}{%
\begin{tabular}{@{}l c c r@{\;}l r@{\;}l r@{\;}l r@{\;}l r@{\;}l r@{\;}l r@{\;}l r@{\;}l r@{\;}l@{}}
\toprule
\multirow{2}{*}{\textbf{Critic}} & \multirow{2}{*}{$k$} & \multirow{2}{*}{\textbf{FB}} & \multicolumn{2}{c}{\multirow{2}{*}{\textbf{Res.\ (\%)}}} & \multicolumn{2}{c}{\multirow{2}{*}{\textbf{Sub.\ (\%)}}} & \multicolumn{2}{c}{\textbf{Res.\ on}} & \multicolumn{2}{c}{\multirow{2}{*}{\textbf{Steps}}} & \multicolumn{2}{c}{\multirow{2}{*}{\textbf{Loc.\ (\%)}}} & \multicolumn{2}{c}{\multirow{2}{*}{\textbf{Loop (\%)}}} & \multicolumn{2}{c}{\multirow{2}{*}{\textbf{Agent~\$}}} & \multicolumn{2}{c}{\multirow{2}{*}{\textbf{Critic~\$}}} & \multicolumn{2}{c}{\multirow{2}{*}{\textbf{Total~\$}}} \\
 & & & \multicolumn{2}{c}{} & \multicolumn{2}{c}{} & \multicolumn{2}{c}{\textbf{Sub.\ (\%)}} & \multicolumn{2}{c}{} & \multicolumn{2}{c}{} & \multicolumn{2}{c}{} & \multicolumn{2}{c}{} & \multicolumn{2}{c}{} & \multicolumn{2}{c}{} \\
\midrule
\multirow{2}{*}{No critic}        & ---  & {\color{gray}\ding{55}} & 28.8 &              & 89.0 &              & 32.4 &              & 34.5 &              & 71.2 &              & 11.6 &              & 0.08 &              & 0.00 &              & 0.08 &              \\
                                  & ---  & \ding{51}              & 29.2 &              & 92.6 &              & 31.5 &              & 42.1 &              & 73.6 &              & 13.6 &              & 0.12 &              & 0.00 &              & 0.12 &              \\
\cmidrule(lr){2-21}
\multirow{4}{*}{\texttt{Opus 4.6} (H)}     & 5    & {\color{gray}\ding{55}} & 51.0 & \dup{22.2}   & 91.4 & \dup{2.4}    & 55.8 & \dup{23.4}   & 38.6 & \dupR{4.1}   & 80.8 & \dup{9.6}    & 25.2 & \dupR{13.6}  & 0.10 & \dupR{0.02}  & 0.96 & \dupR{0.96}  & 1.06 & \dupR{0.98}  \\
                                  & 5    & \ding{51}              & 51.4 & \dup{22.2}   & 98.4 & \dup{5.8}    & 52.2 & \dup{20.7}   & 42.3 & \dupR{0.2}   & 85.6 & \dup{12.0}   & 25.2 & \dupR{11.6}  & 0.12 & \dzero       & 0.96 & \dupR{0.96}  & 1.07 & \dupR{0.95}  \\
                                  & 10   & {\color{gray}\ding{55}} & 47.2 & \dup{18.4}   & 93.4 & \dup{4.4}    & 50.5 & \dup{18.1}   & 39.0 & \dupR{4.5}   & 81.0 & \dup{9.8}    & 23.2 & \dupR{11.6}  & 0.09 & \dupR{0.01}  & 0.97 & \dupR{0.97}  & 1.07 & \dupR{0.98}  \\
                                  & 10   & \ding{51}              & 47.6 & \dup{18.4}   & 98.8 & \dup{6.2}    & 48.2 & \dup{16.7}   & 42.0 & \ddnG{0.1}   & 84.8 & \dup{11.2}   & 23.2 & \dupR{9.6}   & 0.10 & \ddnG{0.02}  & 0.97 & \dupR{0.97}  & 1.08 & \dupR{0.95}  \\
\cmidrule(lr){2-21}
\multirow{4}{*}{\texttt{Opus 4.6} (D)}     & 5    & {\color{gray}\ding{55}} & \textbf{65.0} & \dup{36.2} & 99.8 & \dup{10.8} & \textbf{65.1} & \dup{32.7} & \textbf{30.2} & \ddnG{4.3} & \textbf{91.6} & \dup{20.4} & 9.2 & \ddnG{2.4} & \textbf{0.04} & \ddnG{0.04} & 0.59 & \dupR{0.59} & 0.63 & \dupR{0.55} \\
                                  & 5    & \ding{51}              & \textbf{65.0} & \dup{35.8} & \textbf{100.0} & \dup{7.4} & 65.0 & \dup{33.5} & \textbf{30.2} & \ddnG{11.9} & \textbf{91.6} & \dup{18.0} & \textbf{9.2} & \ddnG{4.4} & \textbf{0.04} & \ddnG{0.08} & 0.59 & \dupR{0.59} & 0.63 & \dupR{0.51} \\
                                  & 10   & {\color{gray}\ding{55}} & 55.8 & \dup{27.0}   & 99.0 & \dup{10.0}   & 56.4 & \dup{24.0}   & 32.7 & \ddnG{1.8}   & 89.4 & \dup{18.2}   & 14.2 & \dupR{2.6}   & 0.06 & \ddnG{0.02}  & \textbf{0.49} & \dupR{0.49} & \textbf{0.55} & \dupR{0.46} \\
                                  & 10   & \ding{51}              & 55.8 & \dup{26.6}   & 99.6 & \dup{7.0}    & 56.0 & \dup{24.5}   & 33.3 & \ddnG{8.8}   & 90.0 & \dup{16.4}   & 14.4 & \dupR{0.8}   & 0.06 & \ddnG{0.06}  & \textbf{0.49} & \dupR{0.49} & \textbf{0.55} & \dupR{0.42} \\
\bottomrule
\end{tabular}%
}
\caption{\texttt{Opus 4.6} teacher on \texttt{CWM-32B}, swept across prompt (H/D), $k\in\{5,10\}$, and fallback. Arrows vs.\ the matching no-critic row at the same fallback state. \textbf{Bold} = best per metric across Opus rows. \ding{51} = fallback to base run~0 (no-critic + \ding{51} uses run~0 $\to$ run~1).}
\label{tab:fallback_full}
\end{table*}

\paragraph{Opus prompt and budget effects.} The detailed prompt (D) dominates the high-level prompt (H) on every metric at both $k$ values: under fallback at $k{=}5$, D reaches 65.0\% resolve vs.\ H's 51.4\%, with shorter trajectories (30.2 vs.\ 42.3 steps), higher localization (91.6 vs.\ 85.6\%), lower stuck-in-loop rate (9.2 vs.\ 25.2\%), and lower agent cost (\$0.04 vs.\ \$0.12). The detailed prompt's per-step instructions appear to give the agent enough scaffolding to converge faster, which more than offsets the longer critic prompt: total cost is \$0.63 (D) vs.\ \$1.07 (H), a $\sim\!1.7\times$ saving despite higher resolve rate. Within each prompt, $k{=}5$ outperforms $k{=}10$ on resolve (51.4 vs.\ 47.6 for H; 65.0 vs.\ 55.8 for D), so more frequent intervention is worth the additional critic calls when the critic itself is strong. Fallback adds only a small bump for Opus (which already submits on $\geq\!91\%$ of tasks) compared to the much larger bump it provides for the trained critic in App.~\ref{app:fallback_triagent}.
