# Supplementary material for: Steer, Don't Solve: Training Small Critic Models for Large Code Agents
Source: arXiv:2606.21811 source file (2026-09-01)
Supplement: Supplementary file 2 [file appendix_fallback_triagent.tex]

\section{Cross-Agent-Model Fallback Ablation}
\label{app:fallback_triagent}

Table~\ref{tab:fallback_triagent} reports the cross-agent-model fallback ablation across three agent models with nine diagnostic metrics; App.~\ref{app:fallback_full} complements it by sweeping the \opus{} teacher across prompt format and $k$ on \cwm. The agent models are \cwm{} (the main-paper agent), \qwenNext, and \qwenThirtyTwoB. For each we report the no-critic baseline, the untrained \qwenEightB{} critic, our trained critic (``Ours'' = \qwenEightB{} trained on teacher critiques generated with the high-level prompt; \cwm{}-only training data on the \cwm{} agent, \cwm{} + \qwenNext{} mix on the two Qwen agents), and the \opus{} teacher critic, all with and without base-run fallback. ``Sub.''\ is the submission rate; ``Res.\ on Sub.''\ is resolve rate computed only over the submitted runs (resolved divided by submitted); ``Steps'' is the average trajectory length in agent steps; ``Loc.''\ is the localization rate (the fraction of tasks where the agent visits one of the gold patch's files); ``Loop'' is the fraction of trajectories flagged stuck-in-loop by the trajectory analyzer; ``Agent~\$'' and ``Critic~\$'' are the average per-instance costs of the agent and the critic respectively, in US dollars; ``Total~\$'' is their sum. Arrows show the direction of change vs.\ the matching no-critic baseline at the same fallback state.

\input{tables/fallback_triagent}


\paragraph{Cross-agent-model observations.} The trained critic improves resolve rate over the no-critic + fallback baseline on all three agent models: \cwm{} 33.0 vs.\ 29.2 ($+3.8$, Ours at $k{=}10$), \qwenNext{} 25.2 vs.\ 20.8 ($+4.4$, Ours at $k{=}10$), and \qwenThirtyTwoB{} 14.8 vs.\ 9.6 ($+5.2$, Ours at $k{=}5$). The \opus{} teacher at $k{=}5$ is the upper bound on each agent model (51.4 / 38.2 / 27.4) and remains substantially above the trained critic in every case, mirroring the gap reported in Table~\ref{tab:main}. The untrained \qwenEightB{} critic under the detailed prompt ties or trails the no-critic baseline on every agent model where it has been measured: on \cwm{} it drops to 27.0 / 29.2 (vs.\ 28.8 / 29.2), on \qwenNext{} it is essentially flat ($20.4$ to $20.6$ vs.\ $20.0$ to $20.8$), and on \qwenThirtyTwoB{} it trails the no-critic baseline at the matching fallback state (9.0 / 10.4 vs.\ 8.8 / 9.6, with the $k{=}5$ + fb row notably below baseline). The Agent~\$ / Critic~\$ split shows that the trained critic adds only \$0.003 to \$0.010 of critic compute per instance on every agent model, while the \opus{} teacher adds \$0.15 to \$0.96 depending on the agent model; the resolve-rate gap to \opus{} therefore comes at a $30\times$ to $92\times$ critic-cost premium (Critic~\$ ratios from Table~\ref{tab:fallback_triagent}: \cwm{} $0.9576/0.0104{=}92{\times}$, \qwenNext{} $0.1539/0.0025{=}62{\times}$, \qwenThirtyTwoB{} $0.2408/0.0080{=}30{\times}$; comparing the main Ours row to Opus k{=}5+fb on each agent model). On \qwenNext{} the trained critic also reduces stuck-in-loop rate, average trajectory length, and per-instance agent cost relative to the no-critic baseline; on \cwm{} the trained critic increases trajectory length and stuck-in-loop rate even as resolve rate improves, indicating that on this agent model the additional steps the critic induces are productive.
